# Supplementary material for: Science Requirements and Detector Concepts for the Electron-Ion Collider: EIC Yellow Report
Source: arXiv:2103.05419 source file (2021-10-27)

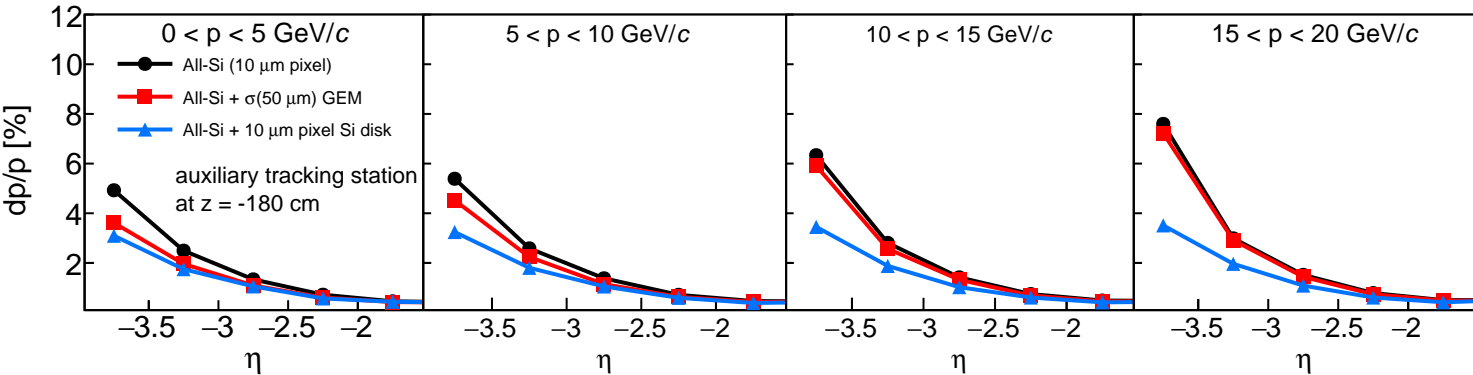

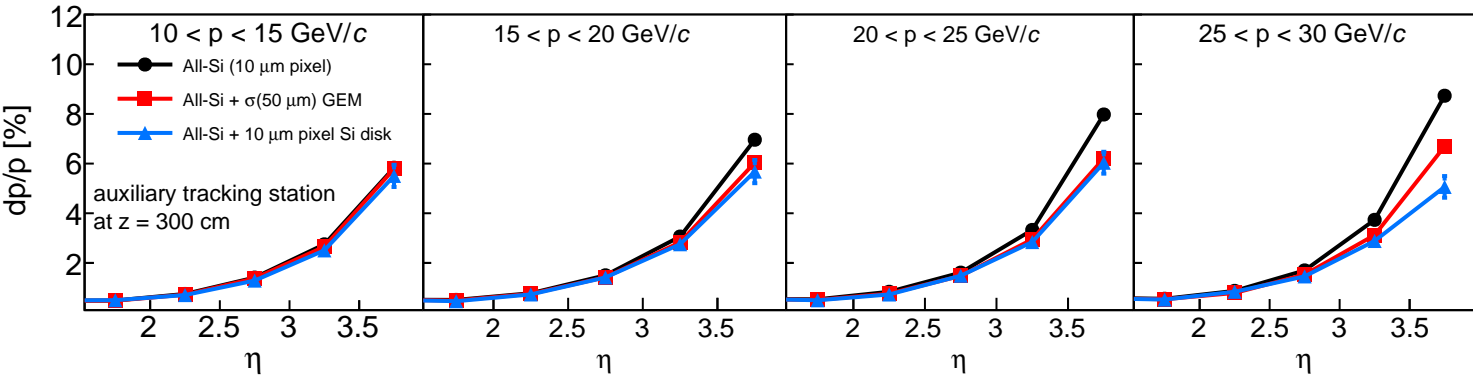

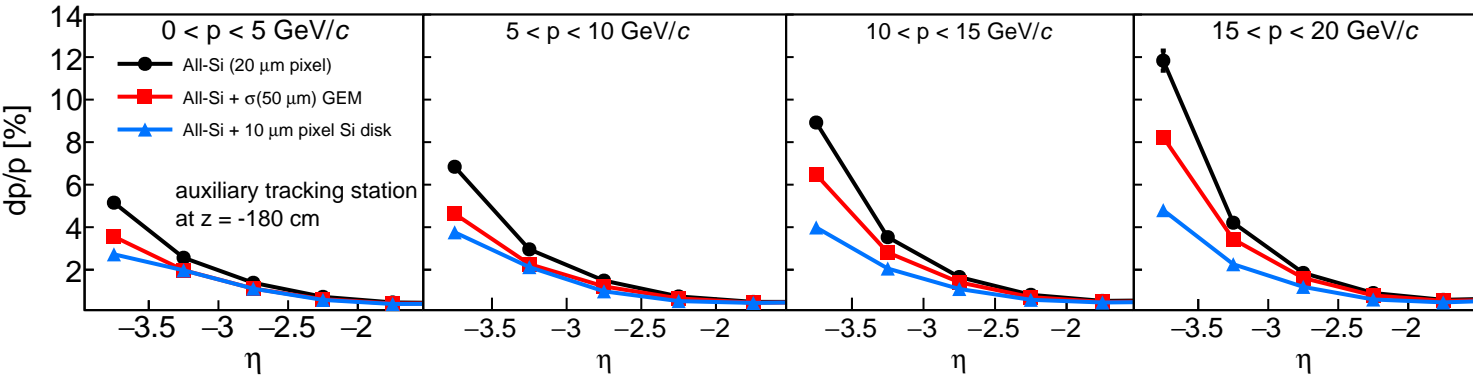

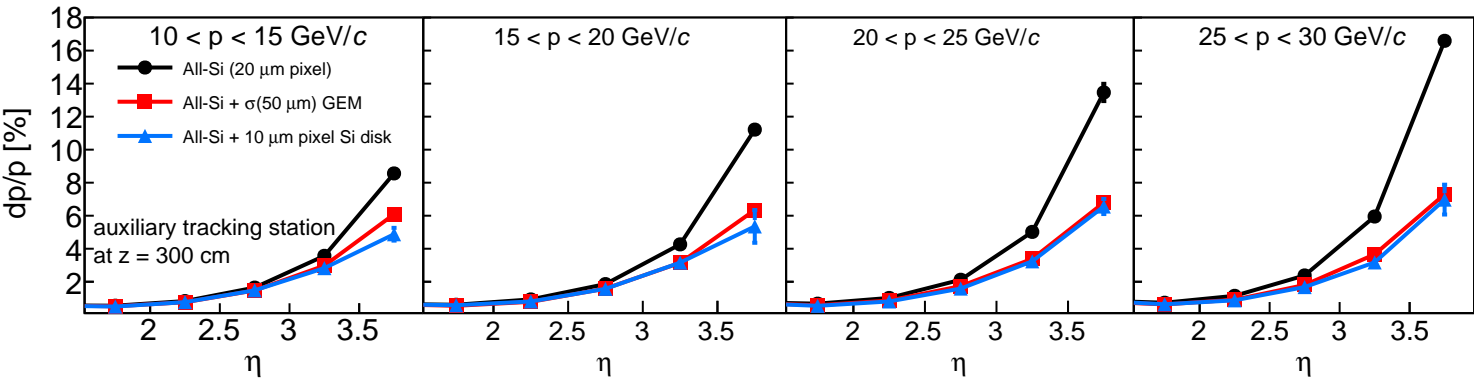

Supplement: Supplementary file 1 [file results_plots_for_YR_new.pdf]
